# Supplementary material for: A Trembling House of Cards? Mapping Adversarial Attacks against Language Agents
Source: arXiv:2402.10196 source file (2024-02-15)
Supplement: Supplementary file 1 [file appendix.tex]

\appendix
\onecolumn

\section{Other Types of Agents}
\label{other_agent}

\textbf{Embodied Agents.}
The objective of embodied agents is to develop entities like robots that can learn to innovatively tackle complex tasks involving engagement with their surroundings. SayCan~\citep{ahn2022i} uses a language model to supply high-level semantic knowledge about the task and take the robot as ``hands and eyes''. \citet{huang2022language} map LLM instructions precisely to admissible actions in the environments by demonstration and proper translations. To reduce spurious correlation between goals and steps stored in pre-trained LLM, \citet{lu2023neurosymbolic} propose neuro-symbolic procedural PLANner with commonsense-infused prompting by the help from commonsense knowledge bases. By addressing the limitation of static plans against dynamic environments and the unrealistic assumption of observing all candidate actions, LLM-Planner~\citep{song2023llm} adopts hierarchical planning methods composed by a high-level and a low-level planner. Besides, \citet{huang2022inner} find that inner monologue allows LLM to richly and precisely process in embodied context over feedback in the form of natural language. However, free-form text may contain impossible actions on a given robot in the current situation, ProgPrompt~\citep{progprompt} presents a programmatic LLM prompt structure to enable plan generation functional across situated environments. It can achieve a significant success rate in VirtualHome household tasks. More recently, \citet{wang2023voyager} introduce \textsc{Voyager} that enables an embodied lifelong agent in Minecraft to select, craft, and add tools in skill libraries from scratch based on feedback from the environment.\\

\noindent
\textbf{Multi-modal Agents.}
In this section, we talk about the existing development of multi-modal agents for comprehensiveness. Going beyond the constraints of purely textual communication, imagery, video and auditory modalities encompass a wide range of valuable signals, enabling language agents to engage with the world in a more direct and nuanced manner. CogAgent~\citep{hong2023cogagent} introduces a medium-sized vision language model specializing in GUI navigation with two tuned low and high-resolution image encoders. \citet{zhang2023appagent} present AppAgent designed for smartphone application operations. It involves creating a comprehensive reference document for an application, which is then leveraged for effective app navigation. \citet{chen2023endtoend} incorporate GPT-4V as the visual perception and cognition module to enhance decision-making. More recently, SeeAct~\citep{zheng2024gpt4vision} demonstrates the potential of GPT-4V as a generalist web agent. Using oracle grounding, GPT-4V could complete 50\% of tasks on live websites without specific fine-tuning. Expanding beyond the scope of image and text modalities, \citet{paul2022avlen} and \citet{gan2020look} delve into the navigation under the bask framework, which includes a dynamic planner that uses visual and auditory observations alongside spatial memories. \citet{yang2023mmreact} integrate X-decoder, VideoBert, and SpeechBERT for image, video, and audio modalities association and processing respectively. Agents with richer perception units can be equipped with diverse perception modules, such as GPS~\citep{parkinson1996progress}, 3D point cloud maps~\citep{schwarz2010mapping}, or non-verbal pointing instructions~\citep{liu2023interngpt}.
